# Supplementary material for: GlossGau: Efficient Inverse Rendering for Glossy Surface with Anisotropic Spherical Gaussian
Source: arXiv:2502.14129 source file (2025-02-19)
Supplement: Supplementary file 1 [file X_suppl.tex]

\clearpage
\setcounter{page}{1}
\maketitlesupplementary
\appendix

\begin{figure*}
\vspace{-1ex}
    \centering
    \scalebox{0.8}{\includegraphics[width=\linewidth]{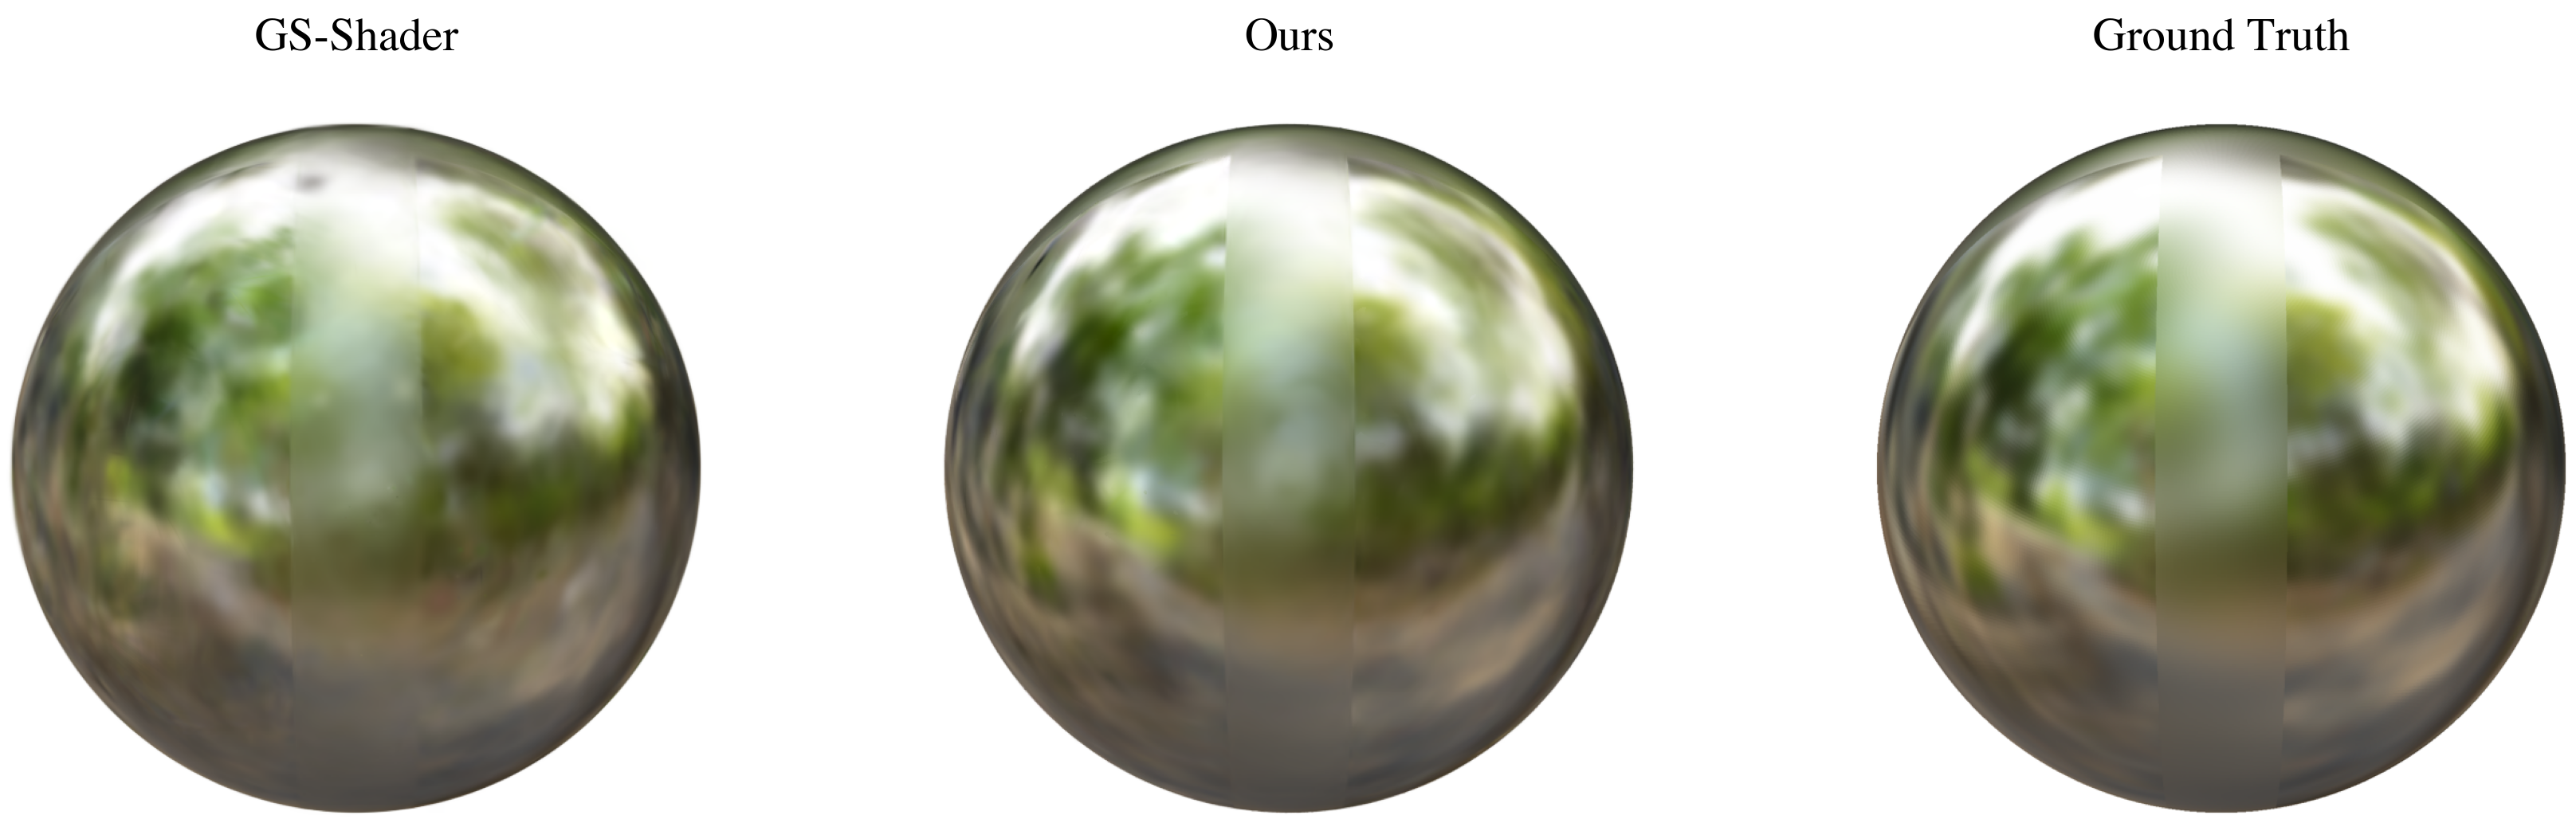}}
    \caption{Visualized comparisons on ``Ball'' category of Shiny Blender Dataset~\cite{verbin2022ref}.
    }
    \label{fig:ball}
    % \vspace{-2ex}
\end{figure*}

\begin{figure*}
\vspace{-1ex}
    \centering
    \scalebox{1}{\includegraphics[width=\linewidth]{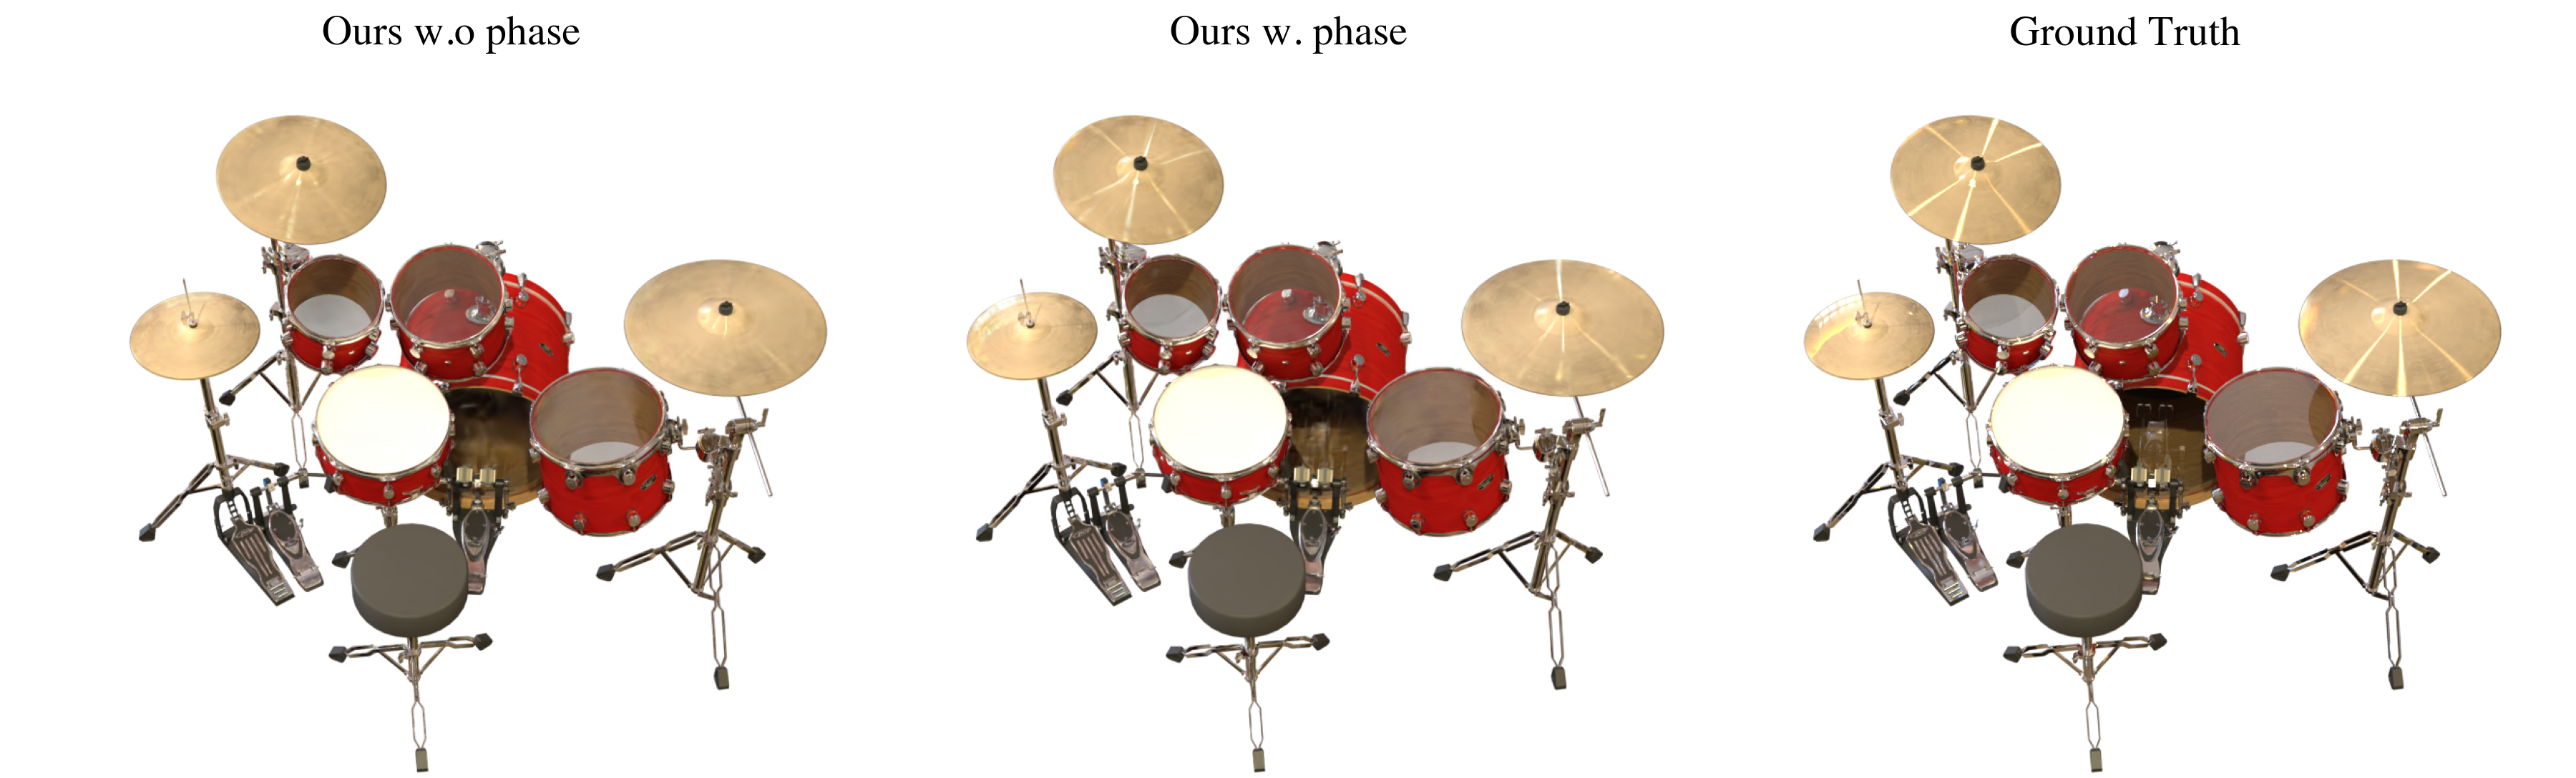}}
    \caption{Visualized comparison between result derived from phased training and result without phased training.}
    \label{fig:ablate}
    % \vspace{-2ex}
\end{figure*}

\begin{table}
\centering
\caption{Quantitative comparisons on Shiny Blender Dataset. We report color each cell as \colorbox{yzybest}{best}, \colorbox{yzysecond}{second best} and \colorbox{yzythird}{third best}.}
\vspace{-1ex}
\scalebox{0.75}{
\begin{tabular}{lcccccc}
\hline
        \multicolumn{7}{c}{Shiny Blender~\cite{verbin2022ref}}       \\
            & \multicolumn{1}{l}{Car} & \multicolumn{1}{l}{Coffee} & \multicolumn{1}{l}{Helmet} & \multicolumn{1}{l}{Teapot} & \multicolumn{1}{l}{Toaster} & \multicolumn{1}{l}{Avg.}           \\ \hline
\multicolumn{7}{c}{PSNR$\uparrow$}                                                                                                                                                                                                                                               \\ \hline
2D-GS~\cite{Huang2DGS2024}        & 27.16                     & \cellcolor{yzythird}32.30                    & 27.29                    & \cellcolor{yzythird}44.97                   & 19.77    &  30.30   \\

Scaffold-GS~\cite{lu2024scaffold}      & \cellcolor{yzythird}27.42                     & \cellcolor{yzybest}32.91                     & \cellcolor{yzybest}28.63                    & 44.80                  & \cellcolor{yzythird}22.13     & \cellcolor{yzysecond}31.18                             \\

GS-Shader~\cite{jiang2024gaussianshader}    & \cellcolor{yzybest}28.46     
   & 30.87                 & \cellcolor{yzythird}28.45                     & 43.36                   & \cellcolor{yzybest}23.17              &  \cellcolor{yzythird}30.86                        \\

GS-IR~\cite{liang2024gs} & 25.93 & 31.62 & 25.58 & 41.17 & 19.26 & 28.71 \\

R3DG~\cite{gao2023relightable}    &  26.99                    & 31.16                    &   26.88                 &  \cellcolor{yzysecond}45.57                  &   20.70                      &  30.26                                                                                                                                                                       \\

Ours & \cellcolor{yzysecond}28.32                          & \cellcolor{yzysecond}32.31                         & \cellcolor{yzysecond}28.48                        & \cellcolor{yzybest}46.03        & \cellcolor{yzysecond}23.08                          &  \cellcolor{yzybest}31.44                        \\ \hline

\multicolumn{7}{c}{SSIM$\uparrow$}                                                                                                                                                                                                                                            \\ \hline
2D-GS~\cite{Huang2DGS2024}        & \cellcolor{yzythird}0.933                   & \cellcolor{yzybest}0.972                    & \cellcolor{yzysecond}0.952                   & \cellcolor{yzysecond}0.996                   & 0.886              &  0.948                          \\

Scaffold-GS~\cite{lu2024scaffold}      & 0.927                    & \cellcolor{yzythird}0.970                     & \cellcolor{yzythird}0.951                    & \cellcolor{yzysecond}0.996                  & \cellcolor{yzythird}0.899                          & \cellcolor{yzythird}0.949                            \\

GS-Shader~\cite{jiang2024gaussianshader}    & \cellcolor{yzybest}0.939                     & 0.968                  & \cellcolor{yzybest}0.953                    & \cellcolor{yzythird}0.995                   & \cellcolor{yzybest}0.902                         & \cellcolor{yzysecond}0.951                                    \\

GS-IR~\cite{liang2024gs} & 0.892 & 0.950 & 0.901 & 0.992 & 0.765 & 0.900  \\ 

R3DG~\cite{gao2023relightable}    &  0.929                    & 0.967                    &   0.943                 &  \cellcolor{yzysecond}0.996                  &   0.891                      &  0.939                                                                                                                                                                                                                                                                     \\

Ours & \cellcolor{yzysecond}0.934                         & \cellcolor{yzysecond}0.971                          & \cellcolor{yzybest}0.953                            & \cellcolor{yzybest}0.997                           & \cellcolor{yzysecond}0.900                             &  \cellcolor{yzybest}0.952                                                                                                                                                                                              
 \\ \hline
 
\multicolumn{7}{c}{LPIPS$\downarrow$}                                                                                                                                                                                                                                              \\ \hline
2D-GS~\cite{Huang2DGS2024}        & \cellcolor{yzythird}0.051                     & \cellcolor{yzybest}0.080                     & \cellcolor{yzysecond}0.080                   & \cellcolor{yzysecond}0.008                   & 0.133       &  0.070                      \\

Scaffold-GS~\cite{lu2024scaffold}      & 0.052                     & \cellcolor{yzythird}0.082                     & \cellcolor{yzybest}0.071                 & \cellcolor{yzythird}0.009                  & \cellcolor{yzybest}0.103              & \cellcolor{yzysecond}0.063                  \\

GS-Shader~\cite{jiang2024gaussianshader}    &\cellcolor{yzysecond}0.049                     & 0.086                     & \cellcolor{yzythird}0.088                    & 0.011                   & \cellcolor{yzythird}0.109                        &  \cellcolor{yzythird}0.069                        \\

GS-IR~\cite{liang2024gs}  & 0.075 & 0.105 & 0.158 & 0.021 & 0.216 & 0.115   \\

R3DG~\cite{gao2023relightable}    &  \cellcolor{yzybest}0.048                    & \cellcolor{yzysecond}0.081                    &   0.096                 &  \cellcolor{yzysecond}0.008                  &  0.131                     &  0.072                                                                                                                                                             \\

Ours & \cellcolor{yzybest}0.048                          & \cellcolor{yzybest}0.080                          & \cellcolor{yzybest}0.071                  & \cellcolor{yzybest}0.007                        &  \cellcolor{yzysecond}0.105          & \cellcolor{yzybest}0.062                                                                                                 
 \\ \hline
\end{tabular}
}
\label{tab:tab_shiny}
      \vspace{-2ex}
\end{table}

\section{Anisotropic Spherical Gaussian}
The normal distribution function approximated by an singular Spherical Gaussian~\cite{wang2009all} is defined as
\begin{equation}
    D(\boldsymbol{h}) = G(\boldsymbol{h}; \boldsymbol{n}, \frac{2}{r^2}, \frac{1}{\pi r^2})
\end{equation}
where $r\in[0, 1]$ is the surface roughness. Under the monochrome assumption, the lope amplitude is identical in all dimensions. 

The ASG function~\cite{xu2013anisotropic} is defined as:
\begin{equation}
\begin{aligned}
    G_{asg}(\mathbf{\nu} \: ; \: [\mathbf{x}, \mathbf{y}, \mathbf{z}],[\lambda, \mu], c)= c \cdot \mathrm{S}(\mathbf{\nu} ; \mathbf{z}) \cdot e^{-\lambda(\mathbf{\nu} \cdot \mathbf{x})^{2}-\mu(\mathbf{\nu} \cdot \mathbf{y})^{2}}
\end{aligned}
\end{equation}
where $\nu$ is the unit direction serving as the function input; $\mathbf{x}$, $\mathbf{y}$, and $\mathbf{z}$ correspond to the tangent, bi-tangent, and lobe axis, respectively, and are mutually orthogonal; $\lambda$ and $\mu$ are the sharpness parameters for the $\mathbf{x}$- and $\mathbf{y}$-axis, satisfying $\lambda, \mu>0$; $c$ is the lobe amplitude; $\mathrm{S}$ is the smooth term defined as $\mathrm{S}(\nu ; \mathbf{z}) = \max (\nu \cdot \mathbf{z}, 0)$. 

Therefore, the ASG approximated normal distribution function~\cite{xu2013anisotropic} is defined as 
\begin{equation}
    D(\boldsymbol{h}) = G_{asg}(\boldsymbol{h}; [\mathbf{x}, \mathbf{y}, \boldsymbol{n}], [\frac{2}{r^2},\frac{2}{r^2}], \frac{1}{\pi r^2})
\end{equation}
where $\mathbf{x}$, $\mathbf{y}$ are two arbitrary directions that form a local frame with $\boldsymbol{n}$. After the approximation, we have sharpness parameter for each direction $\mathbf{x}$ and $\mathbf{y}$ with value the same due to the isotropy. 

Similar to \cite{wang2009all}, \cite{xu2013anisotropic} proposes a warping operator that changes the parameter from $\boldsymbol{h}$ to incident light direction $\boldsymbol{\omega}_i$. During the warping, the sharpness of each basis direction is stretched based on the direction of the incident light, creating anisotropic characteristics. The resulting $\textit{D}$ is 
\begin{equation}
    D(\boldsymbol{\omega}_i) = G_{asg}(\boldsymbol{\omega}_i; [\mathbf{x'}, \mathbf{y'}, \mathbf{z'}], [\frac{2}{8r^2(\boldsymbol{\omega}_i \cdot \boldsymbol{n})^2},\frac{2}{8r^2}], \frac{1}{\pi r^2})
\end{equation}
where $\mathbf{x'}$, $\mathbf{y'}$, $\mathbf{z'}$ are the warped orthonormal basis. $\mathbf{z'}$ is defined as the direction of the reflected $\boldsymbol{\omega}_o$ with respect to $\boldsymbol{n}$ and $\mathbf{x'}$ is defined as the direction of $\boldsymbol{n} \times \mathbf{z'}$. 

\section{BVH Bounding Proxy}
Since 2D-GS primitives are primarily thin surfaces, we thereby construct the bounding proxy as an anisotropically scaled icosahedron~\cite{moenne20243d} with a threshold response value $\alpha_{min}$ to reduce the false-positive hit. Staring from the canonical icosahedron, the vertices are stretched to cover the primitives with at least $\alpha_{min}$ response: 
\begin{equation}
  \label{eq:primitive_transform}
  \mathbf{v} = \sqrt{2 \log(\sigma / \alpha_{min})} 
                \mathbf{S} \mathbf{R}^{T} \mathbf{v} + \mathbf{\mu}
\end{equation}
To deal with the degenerated volume due to the surfel-based representation, we adopt the idea of low-pass filter. We set the scaling vector $s_z = 0.01 \cdot \min(s_x, s_y)$ during the BVH construction. Compared with the standard axis-aligned bounds, the scaled icosahedron proxy reduces the BVH query speed by up to 40\%. 

\begin{figure*}[t]
\vspace{-1ex}
    \centering
    \scalebox{1}{\includegraphics[width=\linewidth]{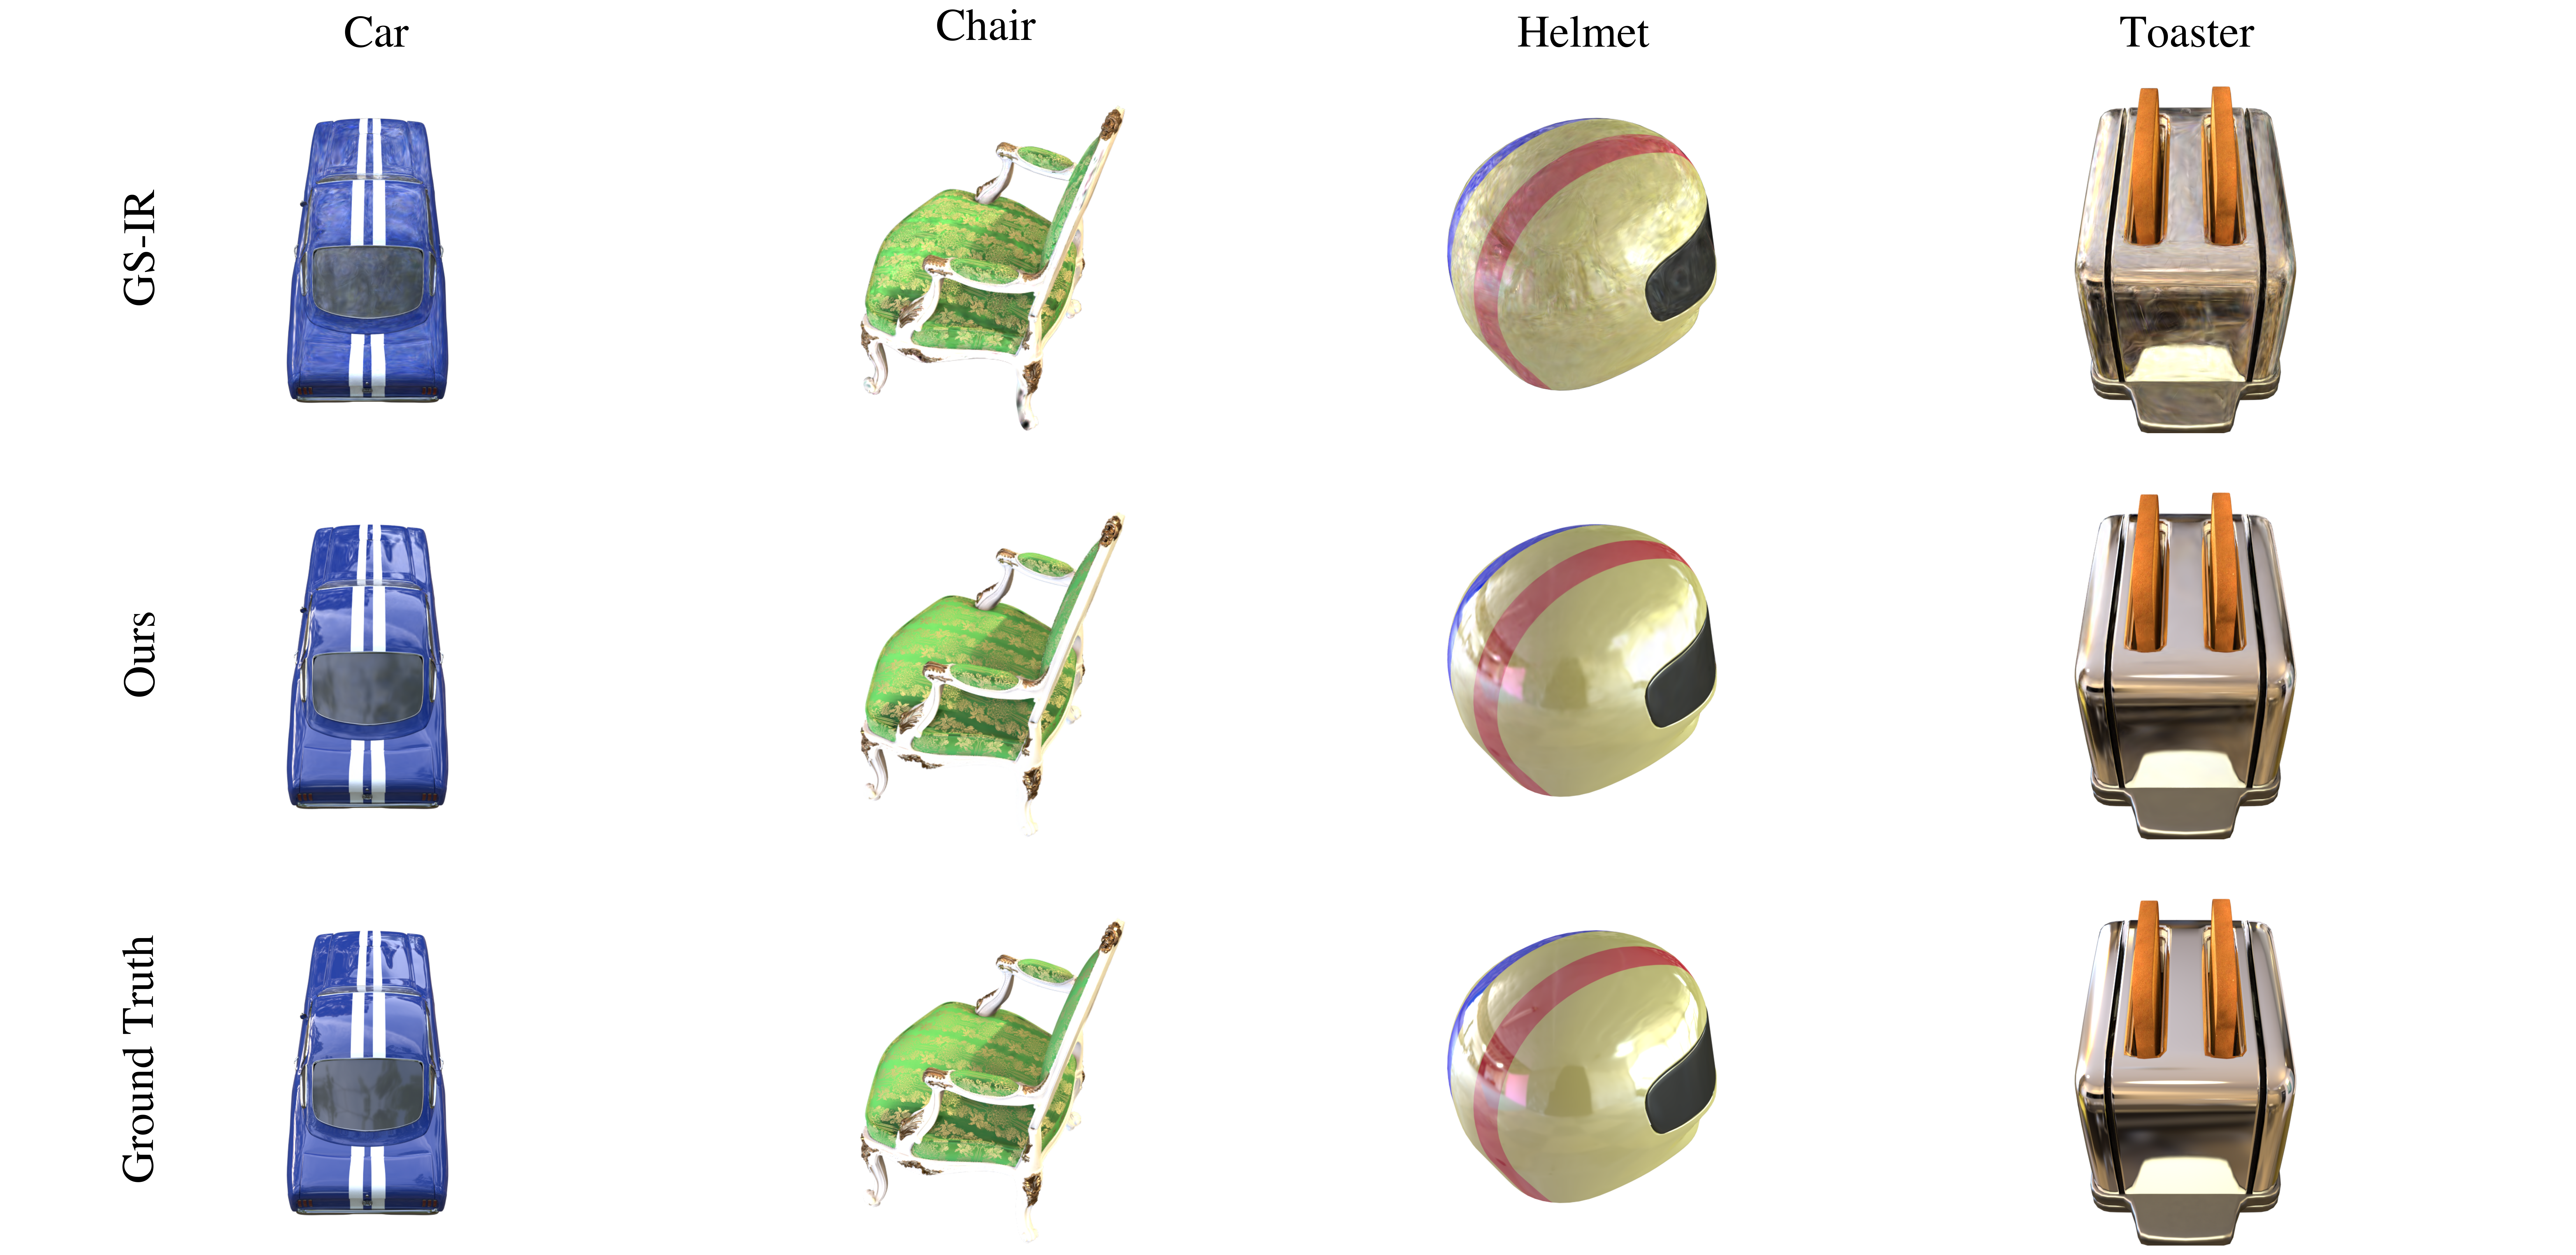}}
    \caption{Visualized comparison with GS-IR~\cite{liang2024gs}}
    \label{fig:gsir}
    % \vspace{-2ex}
\end{figure*}

\section{Additional Results}
\noindent\textbf{Quantitative Results on Shiny Blender~\cite{verbin2022ref}.}
Since R3DG~\cite{gao2023relightable} cannot complete training within the GPU memory of RTX 4090 due to its normal gradient densification strategy and GS-IR~\cite{liang2023gs} fails to generate stable results, we does not include category ``ball'' from the dataset. The quantitative results are reported in Table~\ref{tab:tab_shiny}. The visual comparison of our method with GS-Shader~\cite{jiang2024gaussianshader} on ``Ball'' category is shown in Figure~\ref{fig:ball}. Among the inverse rendering methods, our method demonstrates competitive performance. However, our approach requires much less training and optimization time. Additionally, our method achieves lower LPIPS scores, indicating perceptual quality in the rendered output. 

% which specializes in reflective surface reconstruction, as evidenced on the predominantly reflective Shiny Blender dataset. 

\noindent\textbf{Ablation on Phased Training.}
Instead of implement the phased training, we experiment on optimizing all parameters together from the beginning. The qualitative comparison is shown in Figure \ref{fig:ablate}. We observe that with the phased training, the results exhibit better rendering. 

\noindent\textbf{Qualitative Results.}
GS-IR~\cite{liang2024gs} generates overdensified results with noisy surface, which is quantitatively reflected in the numerical metrics. We show visual comparisons between GS-IR and our method here in Figure~\ref{fig:gsir}. The website accompanied with this supplementary material presents a more interactive comparison for our results. In glossy region, our method achieves comparable reconstruction quality while requiring fewer computational resources. Additionally, our approach better preserves diffuse regions compared to GS-Shader and R3DG, which tend to introduce high-frequency artifacts, whereas our method maintains surface smoothness. We further demonstrate relighting capabilities under varying illumination conditions, applying intensity-modulated environment lighting due to our monochromatic assumption.
